# Supplementary material for: Resonance-enhanced vibrational spectroscopy of molecules on a superconductor
Source: arXiv:2202.08820 ancillary file (2022-02-17)
Supplement: Supplementary file 1 [file SM_2PRL.pdf]

# Supplemental Material for Resonance-enhanced vibrational spectroscopy of molecules on superconductors

Jan Homberg,<sup>1</sup> Alexander Weismann,<sup>1,\*</sup> Troels Markussen,<sup>2</sup> and Richard Berndt<sup>1,†</sup>

<sup>1</sup>*Institut für Experimentelle und Angewandte Physik,  
Christian-Albrechts-Universität zu Kiel, 24098 Kiel, Germany*

<sup>2</sup>*Synopsys Denmark, Fruebjergvej 3, Postbox 4, DK-2100 Copenhagen, Denmark*

## DFT AND DFT-NEGF CALCULATIONS

### Structural relaxation of PbPc on Pb(100)

For the DFT calculations we use a DoubleZetaPolarized basis set and the exchange-correlation functional is described within the generalized gradient approximation (GGA) using the PBE functional [1].

The relaxed structure is shown in Fig. S1. Panel A is a top view illustrating the unit cell containing two PbPc molecules rotated by  $23^\circ$ . Panel B shows a side view of the PbPc monolayer on the Pb(100) surface and an idealized STM tip, which is comprised of a similar Pb(100) surface but with five additional tip atoms. The PbPc monolayer lays almost flat on the Pb(100) surface except the central Pb atom pointing upward. The distance between the flat part of the molecule and the surface is approximately 3.7 Å. The STM tip is positioned right above the Pb atom in the PbPc molecule with a distance of 4.0 Å.

Structural relaxation is performed for the molecules as well as first metal layers plus metal tip atoms until the maximum force is less than 0.05 eV/Å using a  $2 \times 2 \times 1$  Monkhorst Pack  $k$ -point sampling.

### Inelastic DFT-NEGF calculations

To calculate the inelastic signals we use a lowest order expansion (LOE) method [2, 3] going beyond the original wide band approximation [4].

We first calculate the dynamical matrix taking only atoms in the PbPc molecules into account. Although the LOE method allows for scattering with a finite momentum transfer, we limit our calculations

---

\* [weismann@physik.uni-kiel.de](mailto:weismann@physik.uni-kiel.de)

† [berndt@physik.uni-kiel.de](mailto:berndt@physik.uni-kiel.de)

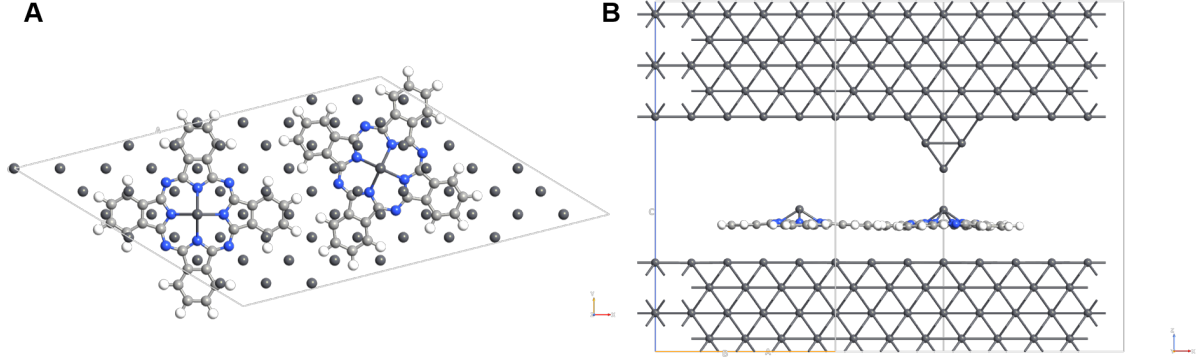

FIG. S1. Calculation cell for the PbPc monolayer on Pb(100). A: Top view of the unit cell containing two PbPc molecules rotated by  $23^\circ$ . B: Side view showing the Pb(100) substrate and tip structure. The tip is positioned directly over the Pb atom of the PbPc molecule. The closest distance between the tip and PbPc molecule is  $4.0 \text{ \AA}$  and the distance from the molecule to the substrate is approximately  $3.7 \text{ \AA}$ .

to only considering incoming and outgoing electrons with transverse momentum  $\mathbf{k}_\parallel = 0$  interacting with phonon also having zero momentum  $\mathbf{q} = 0$ . From the dynamical matrix  $\mathbf{D}$  we obtain the phonon frequencies  $\omega_\lambda$  and eigenvectors  $\mathbf{u}_\lambda$  for a particular phonon band index  $\lambda$ :

$$\mathbf{D}\mathbf{u}_\lambda = \omega_\lambda^2 \mathbf{u}_\lambda, \quad (\text{S1})$$

where the phonon mode vectors are normalized, *i. e.*  $\mathbf{u}^T \cdot \mathbf{u} = 1$ . We further define mass-scaled phonon mode vectors according to

$$\mathbf{v}_\lambda(\alpha) = \mathbf{u}_\lambda(\alpha) \sqrt{\frac{\hbar}{2M_\alpha \omega_\lambda}}, \quad (\text{S2})$$

where  $M_\alpha$  is the mass of the atom with index  $\alpha$ .

The electron-phonon coupling matrix for phonon mode  $\lambda$  is

$$M_\lambda^{\mu\nu} = \langle \phi_\nu | \mathbf{v}_\lambda \cdot \nabla H(r) | \phi_\mu \rangle, \quad (\text{S3})$$

where  $|\phi_{\mu,\nu}\rangle$  denote the LCAO basis orbitals, the derivative of the Hamiltonian is taken with respect to atomic coordinates and restricted to atoms in the PbPc molecules for simplicity. The calculation of the inelastic signals follows the description in [2, 3] and is performed using the InelasticTransmissionSpectrum in QuantumATK.

### Magnetic PbPc on Pb(100)

Since the occurrence of YSR states requires a magnetic moment, we have investigated whether a magnetic configuration can be identified in calculations. For the PBE calculations presented above, this is not the case. Both the free molecule, free monolayer (*i. e.* the molecules in Fig. S1 without the Pb substrate and tip) as well as the PbPc monolayer on Pb(100) give a non-magnetic ground state. In this case, the orbital dominating the transport is the LUMO, which is evident from a projected density of states (PDOS) plot shown in Fig. S2 (A). The spin-resolved PDOS for the PbPc molecule is defined as

$$D^\sigma(E) = \sum_i \sum_{\mu \in \text{PbPc}} w_i |\langle \phi_\mu | \psi_i^\sigma \rangle| \delta(E - \epsilon_i^\sigma) \quad (\text{S4})$$

where the sum over  $i$  runs over all spin  $\sigma$  (up or down) eigenstates  $|\psi_i^\sigma\rangle$  in the system with eigenvalues  $\epsilon_i^\sigma$  including  $k$ -point summation and corresponding weight factors  $w_i$ . The  $\mu$ -sum runs over basis orbitals centered on atoms belonging to the PbPc molecule under the tip. In the calculations, the  $\delta$ -function is replaced by a Gaussian with a width of 0.005 eV.

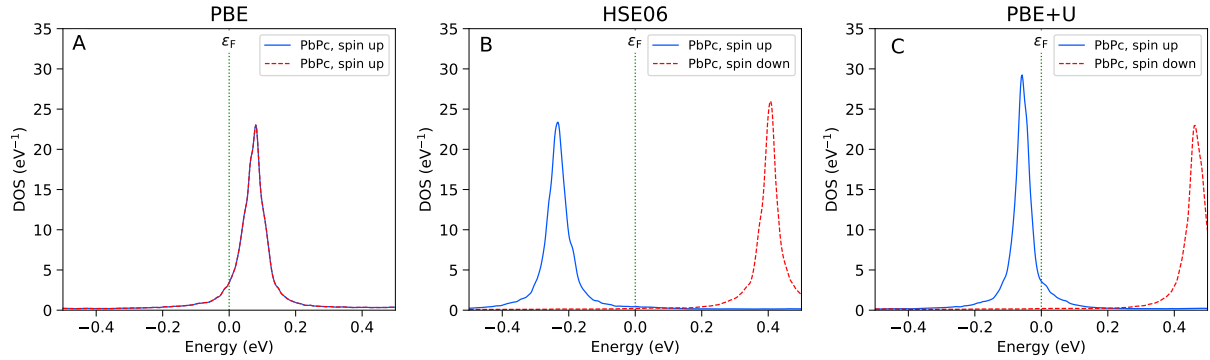

FIG. S2. PDOS of the PbPc molecule under the tip calculated with PBE (A), HSE06 (B), and PBE+U (C). The spin splitting observed with HSE06 and PBE+U is in qualitative agreement with the experimental observation of YSR states.

Interestingly, using the hybrid functional HSE06 [5, 6], the calculated ground state of PbPc molecules on Pb(100) is magnetic as shown in Fig. S2 (B), where a splitting of the spin up and down orbitals close to the Fermi energy is clearly seen. Without the Pb substrate both a single PbPc molecule and the PbPc monolayer come out as non-magnetic with HSE06, showing that the magnetic state of PbPc on Pb(100) is caused by molecule-substrate interaction.

Since inelastic NEGF calculations using hybrid functionals are not yet available in QuantumATK (and, to the best of our knowledge, in other codes), we have also performed DFT+U [7] calculations in order to simulate the magnetic configuration. Figure S2 (C) shows the PDOS from such a PBE+U calculation, where a Hubbard  $U$  energy term has been added to the  $p$ -orbitals on carbon and nitrogen with a  $U$  value of 4 eV. The purpose of PBE+U calculations is not to obtain a one-to-one correspondence with the HSE06 result, but rather a qualitative check of the inelastic PBE calculations. A comparison of PBE and PBE+U inelastic calculations is shown below.

### PBE and PBE+U inelastic calculations

Figure S3 shows the calculated transmission spectrum (left column) and the IETS signal (right column). The transmission spectrum is obtained using the DFT-NEGF method [8]. The IETS signal is here calculated as  $\text{IETS}(V) = \left( \frac{d^2 I}{dV^2} \right) / \left( \frac{dI}{dV} \right)$ . Since we focus on the peak positions, we use a very low temperature of  $T = 1$  K for the IETS calculations to reduce the thermal broadening of the peaks. Panel A shows the transmission spectrum calculated with the PBE functional. The transmission around the Fermi energy ( $E = 0$  eV) is dominated by the spin degenerate LUMO orbital. The corresponding IETS spectrum is displayed in panel C and compared with the experimental results in the main manuscript. Panel B presents the transmission spectrum obtained with the PBE+U functional, where a Hubbard  $U$  has been added to carbon and nitrogen  $p$  orbitals. The transmission spectrum closely resembles the PDOS shown in Fig. S2 (C) with a spin up HOMO orbital closest to the Fermi energy and a spin down LUMO 0.5 eV above the Fermi energy. The IETS spectrum for the PBE+U calculation is shown in panel D. For this calculation, the same vibrational modes and energies have been used as for the PBE calculation. Although there is a notable difference in relative peak intensities between the PBE and PBE+U calculations, the two calculations give qualitatively similar results. In particular, the vibrational modes giving rise to the largest IETS signals appear to be identical in the two calculations. Notice that the spin up HOMO, being almost resonant with the Fermi energy, gives rise to significant peak asymmetries and Fano-like shapes, in agreement with Refs. [2, 3].

Despite the theoretical uncertainty about the magnetic configuration of the PbPc molecules, the qualitative comparison between the PBE and PBE+U IETS spectra shows that the coupling of the vibrational modes to the frontier orbitals is qualitatively similar. This justifies the use of the calculated PBE IETS signal when comparing to the experimental results.

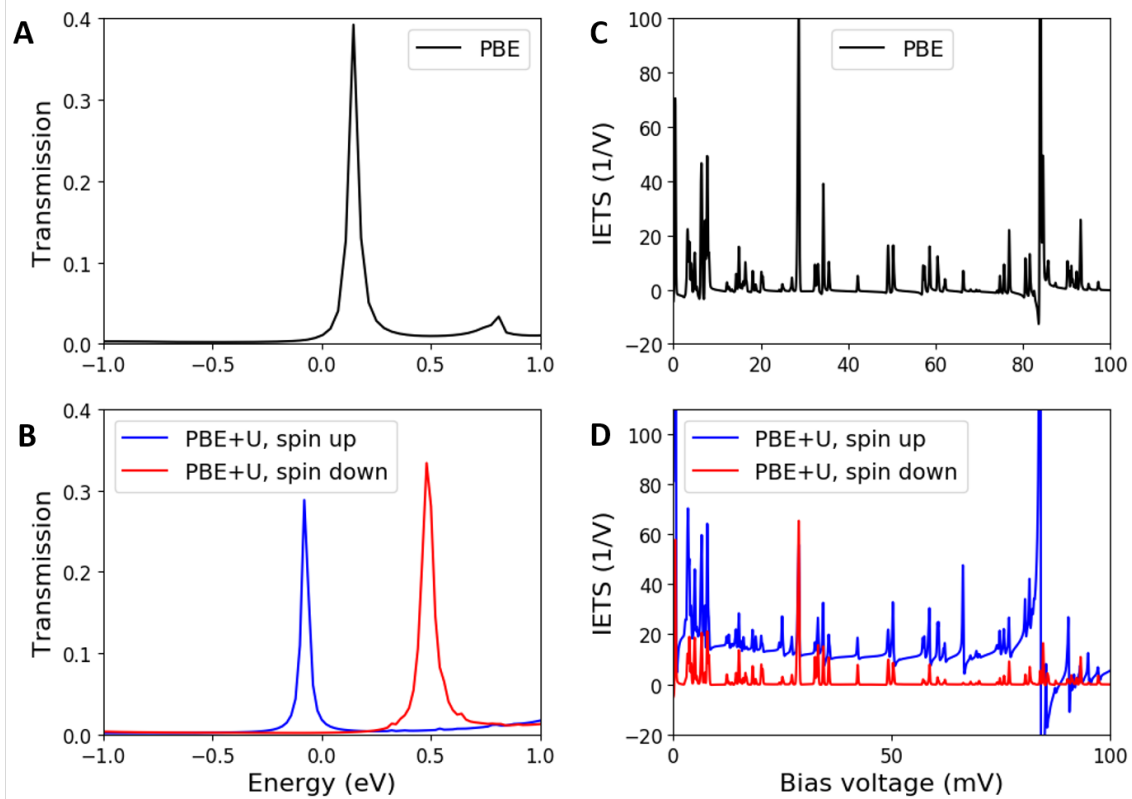

FIG. S3. Transmission spectrum and IETS as obtained using the PBE functional (A) and (C) giving a non-magnetic molecular configuration, and using PBE+U (B) and (D) with a magnetic ground state configuration. For the IETS calculations, we use the same vibrational modes and energies obtained with PBE and focus only on the effect of the different electronic states.

Data from the range  $100 \text{ mV} < |V| < 200 \text{ mV}$

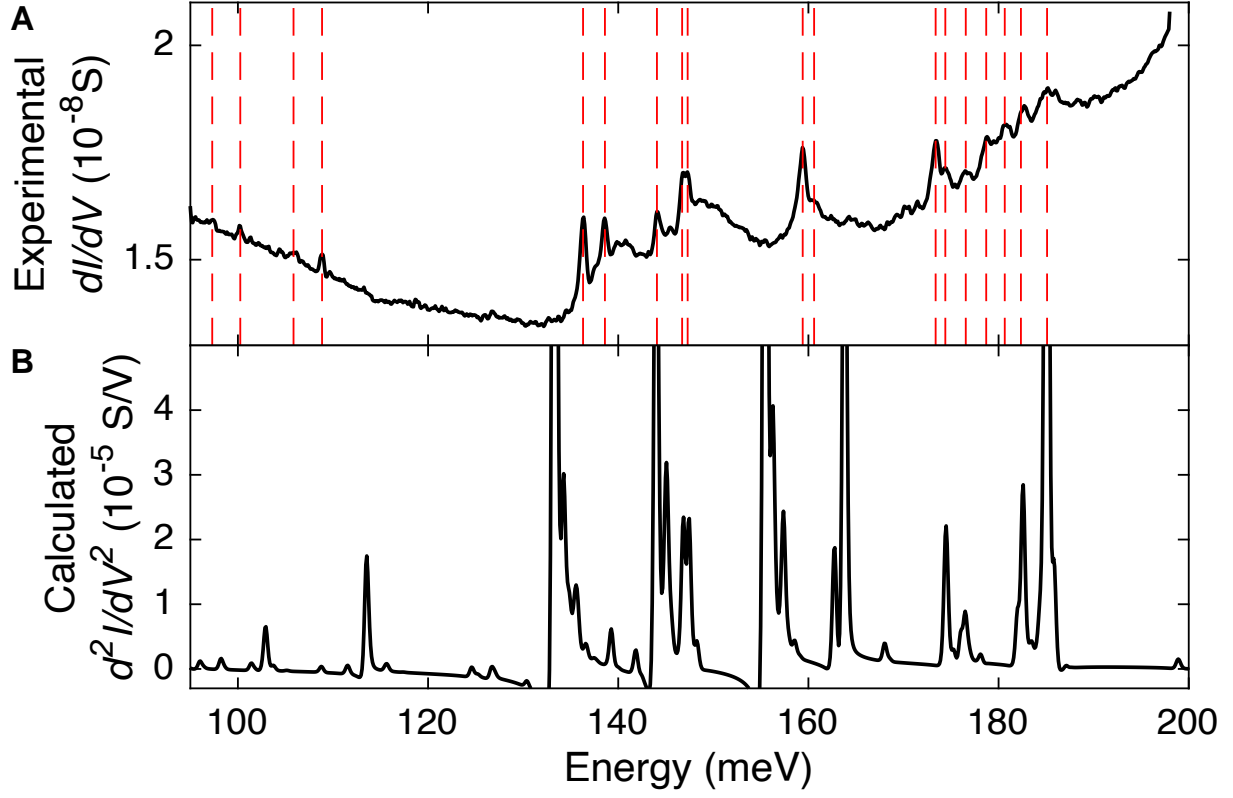

FIG. S4. Experimental and calculated spectra at elevated energies. (A)  $dI/dV$  data shifted by the resonance position  $E_{\text{YSR}} + \Delta_{\text{T}}$ . Vertical lines indicate some of the observed peaks. (B) Calculated spectrum of  $d^2I/dV^2$  shifted by 1.0 meV to higher energies. Based on a tentative peak assignment, we find deviations of less than 7 meV between the experimental and calculated energies. However, the relation between measured and calculated peaks is less obvious than at low energies.

## SUPPLEMENTAL EXPERIMENTAL DATA

## Interaction with neighbor molecules

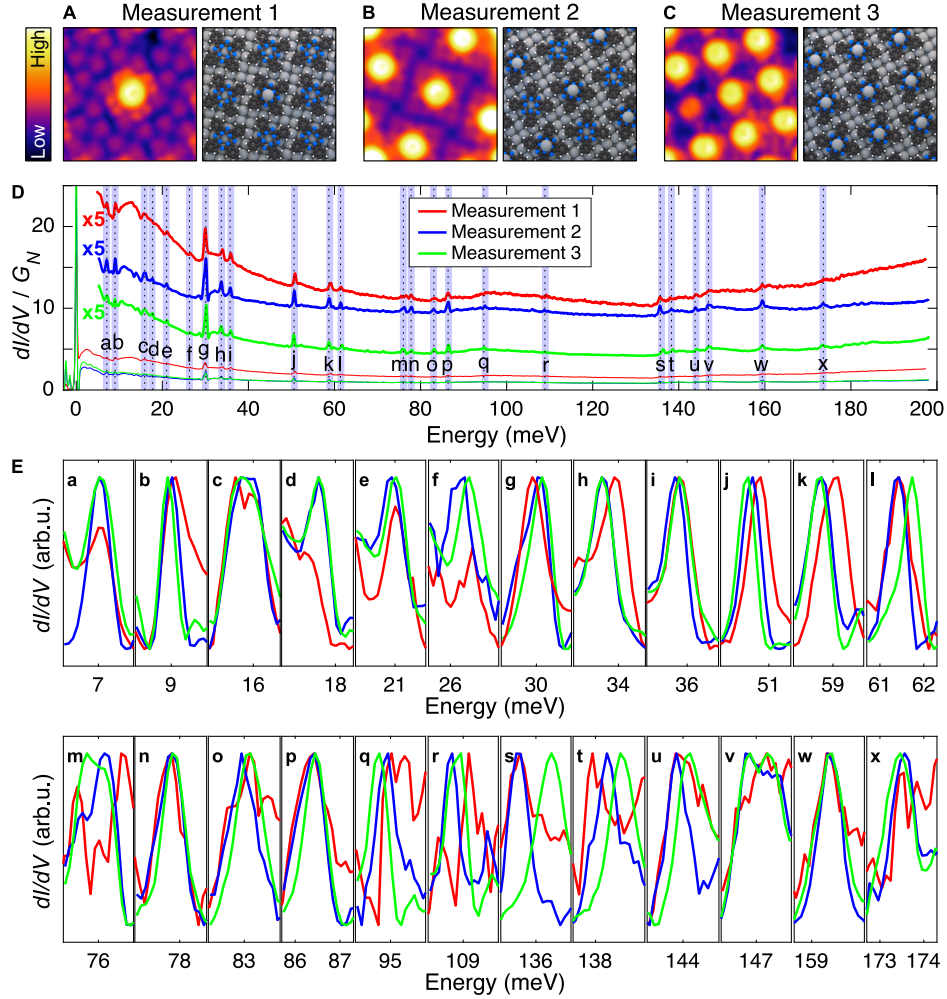

FIG. S5. Topographs and structure models of a PbPc molecule surrounded by (A) Pc without Pb ion, (B) PbPc on next-nearest neighbor (NNN) sites and (C) PbPc on nearest neighbor (NN) and NNN sites. (D)  $dI/dV$  spectra of the central molecules in (A – C) normalized with the conductance  $G_N$  at large energies. Vertical lines indicate the peaks observed from the molecule in (A). (E) Close-up views of peaks indicated by blue shaded areas in (D). Some modes continuously shift to higher (g, n, p, t) or lower (b, j, q) energies as the number of PbPc neighbors increases. Others (h, k) exhibit a red-shift for NNN PbPc that is no further increased by the addition of NN PbPc. The modes in (l) and (s) exhibit a blue-shift only if Pb is present in NN molecules. The modes in (a, c, w) are unaffected by Pb in NN or NNN molecules.

### Interaction with the STM tip

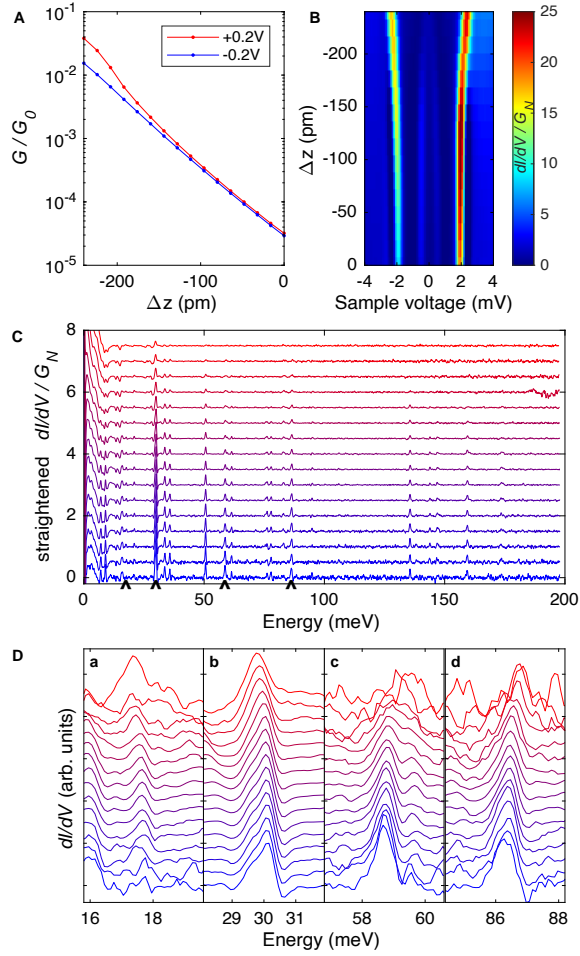

FIG. S6. Vibrational excitations at different tip distances. (A) Evolutions of the conductance at  $V = \pm 0.2\text{ V}$ . The STM current feedback was disabled at  $I = 500\text{ pA}$ , which defines  $\Delta z = 0$ . (B) Low-bias range of 16  $dI/dV$  spectra recorded above the center of a PbPc molecule. From spectrum to spectrum the tip-sample separation was reduced by 16 pm. The YSR peaks shift from  $\approx \pm 1.9$  (bottom spectrum) to  $\approx \pm 2.4\text{ mV}$  during the tip approach. (C)  $dI/dV$  spectra from (A) normalized with the conductance  $G_N$  at large voltages and straightened by removing background features (bulk phonon spectrum and Lorentzian). Only data at  $V > 0$  is shown. The spectra have been shifted by the energy of the relevant YSR peak so that the abscissa shows excitations energies. The top spectrum (red) was recorded at the largest tip-sample separation. Spectra are vertically shifted in steps of  $0.5 G_N$ . (D) Subsections of the untreated spectra showing vibrational peaks at various energies. The data are also presented in Figure 4(a) of the manuscript, where they are normalized to similar peak heights.

### Structure of the PbPc layer

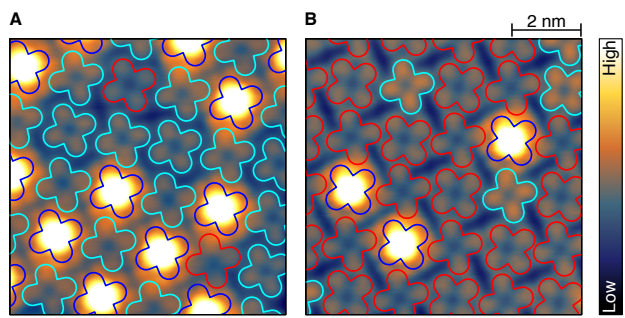

FIG. S7. Constant current topograph of PbPc on Pb(100). (A) and (B) show two different domains. The outlines of the molecules are indicated by lines. PbPc may adsorb with the Pb ion pointing away from the substrate (dark blue lines) or between the substrate and the molecular frame (cyan). In addition, Pc molecules without Pb ion are found (red). The Pb ions may also be intentionally removed by manipulation with the STM tip. YSR resonances are only observed from the first class of molecules. (A)  $V = 6$  mV,  $I = 100$  pA (B)  $V = -6$  mV,  $I = 100$  pA.

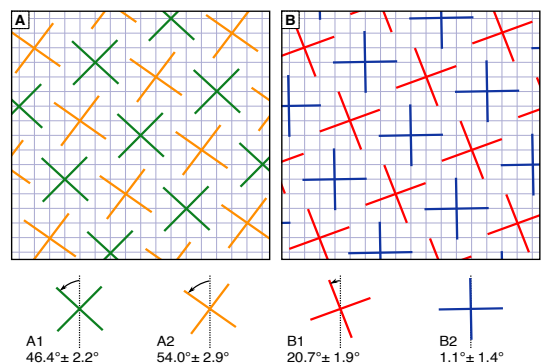

FIG. S8. Schematics of the adsorption geometries. (A) and (B) show the two domains from Figure S7. The Pb(100) lattice is depicted as a square pattern with a mesh size corresponding to 350 pm. Phthalocyanine molecules are indicated by crosses. In both configurations, the molecules are centered atop of a Pb atom and form a  $((3 \times 5)(5 \times 3))$  superstructure with two molecules per unit cell. Colors indicate groups of molecules with different orientations. Angles and their standard deviations were measured from at least 32 molecules per group. The molecules in (A) are oriented with their long axes approximately a  $\langle 001 \rangle$  substrate direction. The orientations of the two groups differ by  $\approx 8^\circ$ . In (B), half of the molecules (blue) have one of their long axes oriented along a  $\langle 011 \rangle$  substrate direction, the other half (red) is rotated by  $\approx 20^\circ$ .

# MODELING OF YSR ENHANCED VIBRATIONAL FEATURES IN $dI/dV$ SPECTRA

To analyze the gating effect on YSR states presented in Figure 4(c) of the manuscript, we calculated spectral line shapes from a set of vibrational mode energies  $\hbar\omega_\nu$  and their cross-sections  $\eta_\nu$  as presented below.

We model the YSR states as a part of the local density of states (LDOS) of the sample using Bogoliubov-de Gennes and Green's function formalisms. The starting point is the homogeneous Green's function of the unperturbed superconducting substrate,

$$G_0(E) = \begin{pmatrix} g(E) & f(E) \\ f^*(-E) & -g^*(-E) \end{pmatrix}, \quad (\text{S5})$$

where  $g(E)$  and  $f(E)$  are the normal and anomalous Green's functions, respectively [9]:

$$g(E) = -\pi\rho_{S,N}(E) \frac{E + i\Gamma}{\sqrt{\Delta_S^2 - (E + i\Gamma)^2}} \quad f(E) = -\pi\rho_{S,N}(E) \frac{\Delta_S}{\sqrt{\Delta_S^2 - (E + i\Gamma)^2}} \quad (\text{S6})$$

Here,  $\rho_{S,N}(E)$  is the LDOS of the sample in the normal conducting state,  $\Delta_S$  the superconducting gap of the sample and  $\Gamma$  a broadening parameter similar to Dynes' parameter. The Green's function matrix is written in spin up electron and spin down hole space. It is identical for spin down electrons and spin up holes. Next, the impurity spin, which acts differently on up-spin and down-spin electrons of the substrate, is included. The respective impurity scattering matrix depends on the electron spin  $\sigma \in \{1, -1\}$ :

$$\Sigma_\sigma = \begin{pmatrix} \sigma JS + W & 0 \\ 0 & \sigma JS - W \end{pmatrix}, \quad (\text{S7})$$

where  $JS$  and  $W$  describe spin dependent and spin independent scattering potentials, respectively. The Green's function of the coupled system reads:

$$G_\sigma(E) = (G_0^{-1}(E) - \Sigma_\sigma)^{-1} \quad (\text{S8})$$

leads to the spin-dependent LDOS:

$$\rho_\sigma(E) = -\frac{1}{\pi} \Im \left( G_\sigma^{(1,1)}(E) \right) \quad (\text{S9})$$

The LDOS of the sample is the sum of both spin components  $\rho_S = \rho_{\text{YSR}}(E) = \rho_\uparrow(E) + \rho_\downarrow(E)$ . Assuming a constant  $\rho_{S,N}(E) = \rho_0$  within the energy range  $-\Delta \dots \Delta$ , it contains YSR states at energies

$$\pm E_{\text{YSR}} = \Delta \frac{\pi^2 \rho_0^2 (J^2 S^2 - W^2) - 1}{\sqrt{(\pi^2 \rho_0^2 (J^2 S^2 - W^2) - 1)^2 + 4\pi^2 \rho_0^2 J^2 S^2}}. \quad (\text{S10})$$

For the density of states of the tip we use the BCS result extended by a Dynes' parameter  $\Gamma$ :

$$\rho_T = \rho_{\text{BCS}}(E) = \rho_{T,N}(E) \cdot \Re \left( \frac{\text{sign}(E) \cdot (E - i\Gamma)}{\sqrt{(E - i\Gamma)^2 - \Delta_T^2}} \right) \quad (\text{S11})$$

$\rho_{T,N}(E)$  is the tip DOS in the normal conducting state and assumed to be constant for simplicity.

The elastic tunneling current  $I_{el}(V)$  is obtained from the DOS of tip and sample:

$$\begin{aligned} I_{el}(V) &= c \int_{-\infty}^{\infty} \rho_t(E - eV) \rho_s(E) [f(E - eV, T) - f(E, T)] dE \\ &= \left( \rho_s(E) * [\rho_t(-E)f(-E, T)] \right)(eV) - \left( [\rho_s(E)f(E, T)] * \rho_t(-E) \right)(eV) \end{aligned} \quad (\text{S12})$$

$f(E, T)$  is the Fermi distribution at a temperature  $T$  and  $c$  is proportional to the tunneling transmission.

For inelastic tunneling, the energy of the final state is lower by the energy  $\hbar\omega_\nu$  of the relevant vibrational mode  $\nu$ :

$$\begin{aligned} I_\nu(V) &= c \eta_\nu \int_{-\infty}^{\infty} dE \left( \rho_t(E - eV + \hbar\omega_\nu) \overbrace{f(E - eV + \hbar\omega_\nu, T)}^{\rightarrow 0, \text{ for } -eV + \hbar\omega_\nu \gg k_B T} \rho_s(E) [1 - f(E, T)] \right. \\ &\quad \left. - \rho_s(E) f(E, T) \rho_t(E - eV - \hbar\omega_\nu) \overbrace{[1 - f(E - eV - \hbar\omega_\nu, T)]}^{\rightarrow 0, \text{ for } eV + \hbar\omega_\nu \gg k_B T} \right) \end{aligned} \quad (\text{S13})$$

Next, the contributions of all vibrational modes, weighed by cross-sections  $\eta_\nu$ , are added to arrive at the inelastic tunneling current:

$$I_{\text{inel}}(V) = \sum_{\nu} I_\nu(V) \quad (\text{S14})$$

Finally, the  $dI/dV$  spectrum is calculated by numerical derivation  $\frac{d}{dV}(I_{el}(V) + I_{\text{inel}}(V))$ .

To account for electronic broadening, the spectrum is furthermore convoluted with a Gaussian with a standard derivation  $\sigma \approx 150 \mu\text{eV}$ . Broadening caused by the voltage modulation  $V_m$  for lock-in detection is taken into account by convolution with the broadening function  $\Re(2\sqrt{V_m^2 - V^2}/(\pi V_m^2))$ .

The best match of the experimentally observed linearly increasing separation between the vibrational features at negative and positive bias was obtained using a constant potential scattering  $\pi\rho_0 W = 0.42$  and an exchange coupling  $\pi\rho_0 JS = 0.57 - 0.88 \cdot V/V$ .

### Calculated vibrational modes

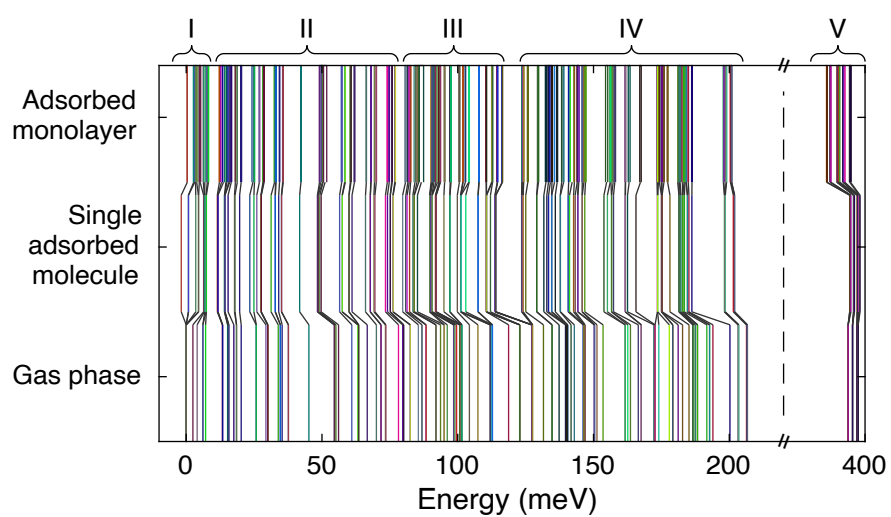

FIG. S9. Energies of vibrational excitations from gas phase, single adsorbed molecule and adsorbed monolayer calculations. Different groups of vibrational modes are identified: (I) frustrated modes and bending modes, (II) higher order bending modes and horizontal rotation of the lobes, (III) lobe squeezing and shearing modes with vertical C-H bending, (IV) C-C and N-C stretching/breathing modes with horizontal C-H bending and (V) C-H stretching modes.

TABLE S1: Properties of calculated vibrations. The unit cell of the calculation contains two PbPc molecules with 57 atoms each, resulting in 342 modes. Modes with energies up to 200 meV are listed below. The symmetry of the vibrations and the dominant direction were analyzed for the molecule below the tip. The dominant direction of motion is indicated by h = exclusively horizontal, hm = mainly horizontal, v = exclusively vertical, vm = mainly vertical, or m = mixed. The symmetry of the vibrations is given by Mulliken symbols denoting the irreducible representations of the point group  $C_{4v}$  of the molecule. Intensities were determined from calculated peak heights in  $d^2I/dV^2$  spectra.

| #  | Energy<br>(meV) | Symmetry<br>(Mulliken) | Dominant<br>Direction | Intensity<br>( $10^{-8}$ S/V) |
|----|-----------------|------------------------|-----------------------|-------------------------------|
| 1  | 0.40            | E                      | h                     | 1547.41                       |
| 2  | 0.41            | E                      | h                     | 1479.81                       |
| 3  | 2.66            | A <sub>2</sub>         | h                     | 65.45                         |
| 4  | 2.87            | A <sub>2</sub>         | hm                    | 164.19                        |
| 5  | 3.15            | E                      | m                     | 444.59                        |
| 6  | 3.16            | E                      | vm                    | 292.41                        |
| 7  | 3.32            | E                      | m                     | 582.47                        |
| 8  | 3.61            | E                      | v                     | 534.36                        |
| 9  | 3.69            | E                      | vm                    | 337.80                        |
| 10 | 4.04            | B <sub>2</sub>         | v                     | 452.65                        |
| 11 | 4.74            | E                      | vm                    | 401.50                        |
| 12 | 4.91            | E                      | vm                    | 373.28                        |
| 13 | 4.92            | E                      | m                     | 141.37                        |
| 14 | 5.34            | A <sub>2</sub>         | vm                    | 116.36                        |
| 15 | 6.25            | B <sub>1</sub>         | v                     | 1314.74                       |
| 16 | 6.42            | E                      | v                     | 901.97                        |
| 17 | 6.50            | E                      | v                     | 886.28                        |
| 18 | 7.22            | A <sub>1</sub>         | v                     | 1120.99                       |
| 19 | 7.69            | E                      | v                     | 1497.28                       |
| 20 | 7.82            | E                      | v                     | 1103.18                       |

TABLE S1: (continued)

| <b>ID</b> | <b>Energy<br/>(meV)</b> | <b>Symmetry<br/>(Mulliken)</b> | <b>Dominant<br/>Direction</b> | <b>Intensity<br/>(<math>10^{-8}</math> S/V)</b> |
|-----------|-------------------------|--------------------------------|-------------------------------|-------------------------------------------------|
| 21        | 8.11                    | B <sub>2</sub>                 | v                             | 519.00                                          |
| 22        | 8.27                    | E                              | v                             | 52.64                                           |
| 23        | 12.16                   | E                              | m                             | 98.83                                           |
| 24        | 12.30                   | E                              | m                             | 85.88                                           |
| 25        | 12.69                   | B <sub>2</sub>                 | h                             | 63.62                                           |
| 26        | 13.32                   | E                              | vm                            | 17.36                                           |
| 27        | 13.39                   | E                              | vm                            | 17.15                                           |
| 28        | 14.10                   | B <sub>1</sub>                 | hm                            | 18.95                                           |
| 29        | 14.32                   | A <sub>2</sub>                 | v                             | 286.07                                          |
| 30        | 14.93                   | E                              | m                             | 354.95                                          |
| 31        | 14.98                   | B <sub>1</sub>                 | m                             | 93.22                                           |
| 32        | 15.01                   | E                              | m                             | 340.83                                          |
| 33        | 15.47                   | B <sub>1</sub>                 | m                             | 99.77                                           |
| 34        | 15.94                   | E                              | m                             | 72.75                                           |
| 35        | 15.99                   | E                              | m                             | 48.87                                           |
| 36        | 16.08                   | E                              | m                             | 46.19                                           |
| 37        | 16.46                   | A <sub>1</sub>                 | v                             | 456.80                                          |
| 38        | 16.74                   | A <sub>1</sub>                 | v                             | 155.78                                          |
| 39        | 18.08                   | E                              | m                             | 184.50                                          |
| 40        | 18.15                   | E                              | m                             | 174.32                                          |
| 41        | 18.79                   | E                              | vm                            | 53.75                                           |
| 42        | 18.82                   | E                              | vm                            | 55.72                                           |
| 43        | 20.10                   | B <sub>1</sub>                 | vm                            | 325.67                                          |
| 44        | 20.39                   | B <sub>1</sub>                 | vm                            | 209.98                                          |
| 45        | 24.22                   | A <sub>2</sub>                 | h                             | 29.17                                           |
| 46        | 24.89                   | B <sub>2</sub>                 | m                             | 113.49                                          |
| 47        | 25.07                   | B <sub>2</sub>                 | m                             | 24.90                                           |
| 48        | 25.21                   | A <sub>2</sub>                 | h                             | 23.33                                           |
| 49        | 26.79                   | B <sub>2</sub>                 | m                             | 47.47                                           |
| 50        | 27.10                   | B <sub>2</sub>                 | m                             | 225.42                                          |
| 51        | 28.19                   | A <sub>1</sub>                 | hm                            | 184.36                                          |

TABLE S1: (continued)

| <b>ID</b> | <b>Energy<br/>(meV)</b> | <b>Symmetry<br/>(Mulliken)</b> | <b>Dominant<br/>Direction</b> | <b>Intensity<br/>(<math>10^{-8}</math> S/V)</b> |
|-----------|-------------------------|--------------------------------|-------------------------------|-------------------------------------------------|
| 52        | 28.37                   | E                              | v                             | 557.24                                          |
| 53        | 28.46                   | E                              | v                             | 1011.44                                         |
| 54        | 28.51                   | E                              | v                             | 720.44                                          |
| 55        | 28.65                   | E                              | v                             | 3169.52                                         |
| 56        | 28.74                   | E                              | v                             | 1905.46                                         |
| 57        | 32.40                   | A <sub>1</sub>                 | vm                            | 479.16                                          |
| 58        | 32.70                   | A <sub>1</sub>                 | vm                            | 122.93                                          |
| 59        | 32.86                   | E                              | m                             | 39.46                                           |
| 60        | 32.92                   | E                              | m                             | 101.67                                          |
| 61        | 33.07                   | E                              | m                             | 233.48                                          |
| 62        | 33.12                   | E                              | m                             | 247.46                                          |
| 63        | 34.29                   | B <sub>1</sub>                 | vm                            | 1899.25                                         |
| 64        | 34.47                   | E                              | vm                            | 9.43                                            |
| 65        | 35.50                   | E                              | m                             | 228.30                                          |
| 66        | 35.57                   | E                              | m                             | 275.47                                          |
| 67        | 35.70                   | E                              | hm                            | 68.21                                           |
| 68        | 35.77                   | E                              | hm                            | 24.50                                           |
| 69        | 42.16                   | A <sub>1</sub>                 | v                             | 264.99                                          |
| 70        | 42.35                   | A <sub>1</sub>                 | v                             | 18.85                                           |
| 71        | 49.02                   | E                              | v                             | 509.65                                          |
| 72        | 49.16                   | E                              | v                             | 477.65                                          |
| 73        | 49.27                   | B <sub>1</sub>                 | v                             | 241.43                                          |
| 74        | 49.93                   | A <sub>2</sub>                 | v                             | 41.72                                           |
| 75        | 50.26                   | A <sub>2</sub>                 | v                             | 133.06                                          |
| 76        | 50.26                   | A <sub>2</sub>                 | v                             | 649.08                                          |
| 77        | 50.36                   | E                              | v                             | 5.43                                            |
| 78        | 50.48                   | A <sub>1</sub>                 | v                             | 146.09                                          |
| 79        | 50.58                   | B <sub>1</sub>                 | v                             | 6.02                                            |
| 80        | 51.75                   | E                              | v                             | 2.42                                            |
| 81        | 57.10                   | B <sub>2</sub>                 | h                             | 499.60                                          |
| 82        | 57.45                   | B <sub>2</sub>                 | h                             | 427.78                                          |

TABLE S1: (continued)

| <b>ID</b> | <b>Energy<br/>(meV)</b> | <b>Symmetry<br/>(Mulliken)</b> | <b>Dominant<br/>Direction</b> | <b>Intensity<br/>(<math>10^{-8}</math> S/V)</b> |
|-----------|-------------------------|--------------------------------|-------------------------------|-------------------------------------------------|
| 83        | 58.34                   | E                              | v                             | 63.83                                           |
| 84        | 58.36                   | E                              | v                             | 56.26                                           |
| 85        | 58.60                   | E                              | v                             | 385.83                                          |
| 86        | 58.62                   | E                              | v                             | 386.43                                          |
| 87        | 60.42                   | E                              | h                             | 314.38                                          |
| 88        | 60.44                   | E                              | h                             | 283.98                                          |
| 89        | 60.66                   | E                              | h                             | 199.33                                          |
| 90        | 60.72                   | E                              | h                             | 70.58                                           |
| 91        | 61.82                   | B <sub>2</sub>                 | v                             | 77.45                                           |
| 92        | 62.12                   | B <sub>2</sub>                 | v                             | 197.01                                          |
| 93        | 66.29                   | B <sub>1</sub>                 | h                             | 339.99                                          |
| 94        | 66.39                   | B <sub>1</sub>                 | h                             | 51.27                                           |
| 95        | 67.95                   | E                              | h                             | 15.31                                           |
| 96        | 68.00                   | E                              | h                             | 14.37                                           |
| 97        | 68.08                   | E                              | h                             | 5.43                                            |
| 98        | 68.13                   | E                              | h                             | 3.97                                            |
| 99        | 69.27                   | A <sub>2</sub>                 | h                             | 30.68                                           |
| 100       | 69.42                   | A <sub>2</sub>                 | h                             | 4.05                                            |
| 101       | 69.93                   | A <sub>1</sub>                 | h                             | 20.60                                           |
| 102       | 70.09                   | A <sub>1</sub>                 | h                             | 9.46                                            |
| 103       | 73.98                   | A <sub>2</sub>                 | hm                            | 29.99                                           |
| 104       | 74.15                   | A <sub>2</sub>                 | hm                            | 35.04                                           |
| 105       | 74.70                   | A <sub>2</sub>                 | vm                            | 309.53                                          |
| 106       | 74.84                   | A <sub>2</sub>                 | vm                            | 0.50                                            |
| 107       | 75.65                   | E                              | m                             | 244.02                                          |
| 108       | 75.66                   | E                              | m                             | 255.48                                          |
| 109       | 75.87                   | E                              | m                             | 4.44                                            |
| 110       | 75.90                   | E                              | m                             | 2.92                                            |
| 111       | 76.82                   | E                              | m                             | 550.61                                          |
| 112       | 76.83                   | E                              | m                             | 582.38                                          |
| 113       | 77.03                   | E                              | m                             | 18.04                                           |

TABLE S1: (continued)

| <b>ID</b> | <b>Energy<br/>(meV)</b> | <b>Symmetry<br/>(Mulliken)</b> | <b>Dominant<br/>Direction</b> | <b>Intensity<br/>(<math>10^{-8}</math> S/V)</b> |
|-----------|-------------------------|--------------------------------|-------------------------------|-------------------------------------------------|
| 114       | 77.06                   | E                              | m                             | 18.78                                           |
| 115       | 80.53                   | E                              | v                             | 660.75                                          |
| 116       | 81.01                   | E                              | v                             | 7.84                                            |
| 117       | 81.52                   | B <sub>1</sub>                 | v                             | 739.86                                          |
| 118       | 81.77                   | A <sub>1</sub>                 | h                             | 114.36                                          |
| 119       | 82.07                   | A <sub>1</sub>                 | h                             | 49.48                                           |
| 120       | 82.23                   | B <sub>2</sub>                 | hm                            | 20.85                                           |
| 121       | 82.54                   | B <sub>2</sub>                 | hm                            | 141.10                                          |
| 122       | 82.76                   | B <sub>2</sub>                 | hm                            | 6.21                                            |
| 123       | 83.94                   | B <sub>1</sub>                 | m                             | 14246.69                                        |
| 124       | 84.55                   | E                              | v                             | 1276.58                                         |
| 125       | 84.64                   | E                              | v                             | 1212.17                                         |
| 126       | 85.29                   | E                              | vm                            | 16.96                                           |
| 127       | 85.54                   | A <sub>1</sub>                 | v                             | 230.30                                          |
| 128       | 85.76                   | E                              | v                             | 208.93                                          |
| 129       | 85.79                   | E                              | v                             | 204.43                                          |
| 130       | 87.43                   | A <sub>1</sub>                 | v                             | 80.49                                           |
| 131       | 90.15                   | E                              | m                             | 267.62                                          |
| 132       | 90.18                   | E                              | m                             | 278.96                                          |
| 133       | 90.47                   | B <sub>1</sub>                 | v                             | 324.83                                          |
| 134       | 90.48                   | E                              | hm                            | 5.55                                            |
| 135       | 90.53                   | E                              | hm                            | 6.10                                            |
| 136       | 91.05                   | E                              | vm                            | 216.48                                          |
| 137       | 91.06                   | E                              | vm                            | 228.09                                          |
| 138       | 91.42                   | A <sub>1</sub>                 | v                             | 175.55                                          |
| 139       | 91.74                   | E                              | v                             | 60.61                                           |
| 140       | 92.23                   | E                              | v                             | 179.38                                          |
| 141       | 92.28                   | E                              | v                             | 184.62                                          |
| 142       | 92.83                   | A <sub>1</sub>                 | v                             | 79.27                                           |
| 143       | 93.07                   | A <sub>2</sub>                 | v                             | 211.41                                          |
| 144       | 93.16                   | E                              | v                             | 412.66                                          |

TABLE S1: (continued)

| <b>ID</b> | <b>Energy<br/>(meV)</b> | <b>Symmetry<br/>(Mulliken)</b> | <b>Dominant<br/>Direction</b> | <b>Intensity<br/>(<math>10^{-8}</math> S/V)</b> |
|-----------|-------------------------|--------------------------------|-------------------------------|-------------------------------------------------|
| 145       | 93.19                   | E                              | v                             | 468.96                                          |
| 146       | 93.23                   | E                              | v                             | 443.22                                          |
| 147       | 93.51                   | A <sub>1</sub>                 | v                             | 2.44                                            |
| 148       | 93.56                   | B <sub>2</sub>                 | v                             | 31.04                                           |
| 149       | 93.63                   | E                              | v                             | 11.14                                           |
| 150       | 93.65                   | E                              | v                             | 8.87                                            |
| 151       | 94.98                   | B <sub>1</sub>                 | h                             | 117.96                                          |
| 152       | 95.35                   | B <sub>1</sub>                 | h                             | 18.20                                           |
| 153       | 97.20                   | E                              | h                             | 82.70                                           |
| 154       | 97.23                   | E                              | h                             | 78.84                                           |
| 155       | 97.53                   | E                              | h                             | 13.09                                           |
| 156       | 97.56                   | E                              | h                             | 12.71                                           |
| 157       | 100.40                  | A <sub>1</sub>                 | h                             | 106.89                                          |
| 158       | 100.81                  | A <sub>2</sub>                 | h                             | 20.84                                           |
| 159       | 101.83                  | E                              | v                             | 189.13                                          |
| 160       | 101.90                  | E                              | v                             | 174.98                                          |
| 161       | 101.92                  | E                              | v                             | 200.48                                          |
| 162       | 102.01                  | E                              | v                             | 149.03                                          |
| 163       | 102.71                  | A <sub>2</sub>                 | h                             | 77.07                                           |
| 164       | 102.92                  | A <sub>2</sub>                 | h                             | 5.80                                            |
| 165       | 104.07                  | E                              | v                             | 3.32                                            |
| 166       | 104.10                  | E                              | v                             | 2.58                                            |
| 167       | 104.16                  | E                              | v                             | 4.82                                            |
| 168       | 104.29                  | E                              | v                             | 2.88                                            |
| 169       | 107.75                  | E                              | h                             | 38.32                                           |
| 170       | 107.80                  | E                              | h                             | 27.83                                           |
| 171       | 107.83                  | E                              | h                             | 22.59                                           |
| 172       | 107.91                  | E                              | h                             | 3.91                                            |
| 173       | 110.43                  | E                              | v                             | 34.47                                           |
| 174       | 110.50                  | E                              | v                             | 35.09                                           |
| 175       | 110.56                  | E                              | v                             | 36.42                                           |

TABLE S1: (continued)

| <b>ID</b> | <b>Energy<br/>(meV)</b> | <b>Symmetry<br/>(Mulliken)</b> | <b>Dominant<br/>Direction</b> | <b>Intensity<br/>(<math>10^{-8}</math> S/V)</b> |
|-----------|-------------------------|--------------------------------|-------------------------------|-------------------------------------------------|
| 176       | 110.61                  | E                              | v                             | 37.51                                           |
| 177       | 112.47                  | B <sub>2</sub>                 | h                             | 991.49                                          |
| 178       | 112.54                  | B <sub>2</sub>                 | h                             | 771.82                                          |
| 179       | 112.65                  | E                              | vm                            | 8.29                                            |
| 180       | 112.75                  | E                              | vm                            | 65.50                                           |
| 181       | 112.79                  | E                              | v                             | 2.67                                            |
| 182       | 112.86                  | E                              | v                             | 0.21                                            |
| 183       | 114.46                  | B <sub>2</sub>                 | v                             | 19.41                                           |
| 184       | 114.58                  | E                              | v                             | 34.79                                           |
| 185       | 114.63                  | E                              | v                             | 37.14                                           |
| 186       | 114.74                  | A <sub>2</sub>                 | v                             | 36.61                                           |
| 187       | 116.33                  | E                              | v                             | 1.70                                            |
| 188       | 116.40                  | E                              | v                             | 1.48                                            |
| 189       | 116.45                  | B <sub>2</sub>                 | v                             | 1.43                                            |
| 190       | 116.50                  | E                              | v                             | 0.62                                            |
| 191       | 123.54                  | A <sub>1</sub>                 | h                             | 119.92                                          |
| 192       | 123.65                  | E                              | h                             | 5.83                                            |
| 193       | 123.70                  | E                              | h                             | 23.66                                           |
| 194       | 123.76                  | E                              | h                             | 5.17                                            |
| 195       | 124.14                  | E                              | h                             | 3.56                                            |
| 196       | 124.19                  | E                              | h                             | 13.06                                           |
| 197       | 124.26                  | E                              | h                             | 20.63                                           |
| 198       | 124.32                  | E                              | h                             | 3.15                                            |
| 199       | 125.65                  | B <sub>2</sub>                 | h                             | 164.52                                          |
| 200       | 125.97                  | B <sub>2</sub>                 | h                             | 66.39                                           |
| 201       | 129.37                  | E                              | h                             | 56.75                                           |
| 202       | 129.42                  | E                              | h                             | 48.17                                           |
| 203       | 129.73                  | E                              | h                             | 10.46                                           |
| 204       | 129.75                  | E                              | h                             | 7.32                                            |
| 205       | 132.27                  | B <sub>1</sub>                 | h                             | 23108.16                                        |
| 206       | 132.71                  | A <sub>2</sub>                 | h                             | 28.64                                           |

TABLE S1: (continued)

| <b>ID</b> | <b>Energy<br/>(meV)</b> | <b>Symmetry<br/>(Mulliken)</b> | <b>Dominant<br/>Direction</b> | <b>Intensity<br/>(<math>10^{-8}</math> S/V)</b> |
|-----------|-------------------------|--------------------------------|-------------------------------|-------------------------------------------------|
| 207       | 133.22                  | B <sub>2</sub>                 | h                             | 2396.57                                         |
| 208       | 133.62                  | A <sub>2</sub>                 | h                             | 33.09                                           |
| 209       | 133.84                  | E                              | h                             | 595.09                                          |
| 210       | 134.41                  | E                              | h                             | 512.73                                          |
| 211       | 134.66                  | E                              | h                             | 320.22                                          |
| 212       | 134.73                  | E                              | h                             | 323.36                                          |
| 213       | 135.57                  | E                              | h                             | 112.11                                          |
| 214       | 135.68                  | E                              | h                             | 107.51                                          |
| 215       | 136.45                  | A <sub>1</sub>                 | h                             | 53.50                                           |
| 216       | 136.78                  | A <sub>1</sub>                 | h                             | 21.35                                           |
| 217       | 138.24                  | E                              | h                             | 296.66                                          |
| 218       | 138.31                  | E                              | h                             | 292.81                                          |
| 219       | 138.95                  | E                              | h                             | 18.89                                           |
| 220       | 139.04                  | E                              | h                             | 14.06                                           |
| 221       | 140.79                  | A <sub>2</sub>                 | h                             | 215.77                                          |
| 222       | 140.93                  | A <sub>2</sub>                 | h                             | 206.47                                          |
| 223       | 141.45                  | A <sub>1</sub>                 | h                             | 71.19                                           |
| 224       | 142.81                  | A <sub>2</sub>                 | h                             | 81.41                                           |
| 225       | 142.92                  | E                              | h                             | 4637.10                                         |
| 226       | 143.00                  | E                              | h                             | 5050.88                                         |
| 227       | 143.92                  | B <sub>2</sub>                 | h                             | 908.89                                          |
| 228       | 144.08                  | E                              | h                             | 1132.39                                         |
| 229       | 144.16                  | E                              | h                             | 1051.70                                         |
| 230       | 144.54                  | E                              | h                             | 171.04                                          |
| 231       | 144.58                  | E                              | h                             | 156.25                                          |
| 232       | 144.61                  | E                              | h                             | 126.90                                          |
| 233       | 145.83                  | E                              | h                             | 983.25                                          |
| 234       | 145.87                  | E                              | h                             | 1159.49                                         |
| 235       | 146.43                  | E                              | h                             | 1163.05                                         |
| 236       | 146.47                  | E                              | h                             | 1030.99                                         |
| 237       | 146.83                  | A <sub>2</sub>                 | h                             | 145.08                                          |

TABLE S1: (continued)

| <b>ID</b> | <b>Energy<br/>(meV)</b> | <b>Symmetry<br/>(Mulliken)</b> | <b>Dominant<br/>Direction</b> | <b>Intensity<br/>(<math>10^{-8}</math> S/V)</b> |
|-----------|-------------------------|--------------------------------|-------------------------------|-------------------------------------------------|
| 238       | 147.29                  | A <sub>2</sub>                 | h                             | 415.26                                          |
| 239       | 154.44                  | B <sub>1</sub>                 | h                             | 19307.37                                        |
| 240       | 155.24                  | B <sub>2</sub>                 | h                             | 3324.53                                         |
| 241       | 155.93                  | B <sub>2</sub>                 | h                             | 53.14                                           |
| 242       | 156.36                  | E                              | h                             | 827.95                                          |
| 243       | 156.37                  | E                              | h                             | 839.22                                          |
| 244       | 156.44                  | E                              | h                             | 390.37                                          |
| 245       | 156.90                  | A <sub>2</sub>                 | h                             | 187.93                                          |
| 246       | 157.56                  | E                              | h                             | 120.20                                          |
| 247       | 157.58                  | E                              | h                             | 107.90                                          |
| 248       | 158.11                  | A <sub>2</sub>                 | h                             | 38.71                                           |
| 249       | 161.69                  | E                              | h                             | 990.57                                          |
| 250       | 161.77                  | E                              | h                             | 756.17                                          |
| 251       | 161.78                  | E                              | h                             | 259.51                                          |
| 252       | 161.83                  | E                              | h                             | 12.04                                           |
| 253       | 162.79                  | B <sub>1</sub>                 | h                             | 10083.63                                        |
| 254       | 163.46                  | E                              | h                             | 43.90                                           |
| 255       | 167.01                  | A <sub>1</sub>                 | h                             | 269.48                                          |
| 256       | 167.59                  | A <sub>1</sub>                 | h                             | 32.73                                           |
| 257       | 173.42                  | E                              | h                             | 775.85                                          |
| 258       | 173.43                  | E                              | h                             | 805.29                                          |
| 259       | 173.55                  | A <sub>1</sub>                 | h                             | 24.12                                           |
| 260       | 173.58                  | E                              | h                             | 414.89                                          |
| 261       | 173.62                  | E                              | h                             | 288.06                                          |
| 262       | 174.17                  | E                              | h                             | 103.64                                          |
| 263       | 174.24                  | E                              | h                             | 87.02                                           |
| 264       | 174.26                  | E                              | h                             | 82.05                                           |
| 265       | 174.97                  | E                              | h                             | 13.26                                           |
| 266       | 175.00                  | E                              | h                             | 415.10                                          |
| 267       | 175.01                  | E                              | h                             | 61.50                                           |
| 268       | 175.47                  | E                              | h                             | 710.48                                          |

TABLE S1: (continued)

| <b>ID</b> | <b>Energy<br/>(meV)</b> | <b>Symmetry<br/>(Mulliken)</b> | <b>Dominant<br/>Direction</b> | <b>Intensity<br/>(<math>10^{-8}</math> S/V)</b> |
|-----------|-------------------------|--------------------------------|-------------------------------|-------------------------------------------------|
| 269       | 175.86                  | E                              | h                             | 95.62                                           |
| 270       | 176.03                  | E                              | h                             | 10.37                                           |
| 271       | 177.11                  | A <sub>1</sub>                 | h                             | 132.37                                          |
| 272       | 177.46                  | A <sub>1</sub>                 | h                             | 0.02                                            |
| 273       | 180.99                  | E                              | h                             | 425.00                                          |
| 274       | 181.01                  | E                              | h                             | 467.34                                          |
| 275       | 181.43                  | A <sub>2</sub>                 | h                             | 44.86                                           |
| 276       | 181.53                  | B <sub>1</sub>                 | h                             | 2211.79                                         |
| 277       | 181.60                  | E                              | h                             | 384.70                                          |
| 278       | 181.63                  | E                              | h                             | 50.61                                           |
| 279       | 181.65                  | E                              | h                             | 44.57                                           |
| 280       | 182.09                  | A <sub>2</sub>                 | h                             | 5.30                                            |
| 281       | 182.46                  | B <sub>2</sub>                 | h                             | 207.14                                          |
| 282       | 183.00                  | E                              | h                             | 31.17                                           |
| 283       | 183.32                  | E                              | h                             | 332.24                                          |
| 284       | 183.38                  | E                              | h                             | 243.86                                          |
| 285       | 183.68                  | E                              | h                             | 33.86                                           |
| 286       | 183.69                  | E                              | h                             | 64.38                                           |
| 287       | 184.01                  | E                              | h                             | 8923.23                                         |
| 288       | 184.12                  | E                              | h                             | 7932.17                                         |
| 289       | 184.15                  | E                              | h                             | 822.16                                          |
| 290       | 184.25                  | E                              | h                             | 32.71                                           |
| 291       | 184.85                  | A <sub>2</sub>                 | h                             | 1591.26                                         |
| 292       | 184.97                  | A <sub>2</sub>                 | h                             | 19.98                                           |
| 293       | 186.13                  | A <sub>1</sub>                 | h                             | 71.30                                           |
| 294       | 186.40                  | A <sub>1</sub>                 | h                             | 13.36                                           |
| 295       | 197.79                  | B <sub>1</sub>                 | h                             | 47.61                                           |
| 296       | 197.86                  | E                              | h                             | 45.13                                           |
| 297       | 197.92                  | E                              | h                             | 33.68                                           |
| 298       | 198.06                  | A <sub>1</sub>                 | h                             | 32.23                                           |
| 299       | 198.81                  | B <sub>1</sub>                 | h                             | 0.83                                            |

TABLE S1: (continued)

| <b>ID</b> | <b>Energy<br/>(meV)</b> | <b>Symmetry<br/>(Mulliken)</b> | <b>Dominant<br/>Direction</b> | <b>Intensity<br/>(<math>10^{-8}</math> S/V)</b> |
|-----------|-------------------------|--------------------------------|-------------------------------|-------------------------------------------------|
| 300       | 198.89                  | E                              | h                             | 1.08                                            |
| 301       | 198.91                  | E                              | h                             | 1.10                                            |
| 302       | 199.08                  | A <sub>2</sub>                 | h                             | 8.40                                            |

### Experimental vibration energies

TABLE S2: Experimental vibration energies. In Fig. 3(a) of the main manuscript and in Fig. S4A, a spectrum revealing a total of 46 inelastic excitations is shown. Here, we list the observed energies and estimated effective cross sections  $\eta$  of the corresponding vibrational modes. Both were obtained by simulating the measured spectrum as described above. In addition, the assigned calculated modes are listed.

| Energy<br>(meV) | $\eta$<br>(%) | Assigned<br>calculated mode # |
|-----------------|---------------|-------------------------------|
| 7.1             | 0.35          | 15-17                         |
| 9.0             | 0.6           | 19-20                         |
| 14.2            | 0.15          | 23-27                         |
| 15.8            | 0.25          | 29-32                         |
| 17.7            | 0.25          | 37-38                         |
| 21.0            | 0.2           | 43-44                         |
| 26.4            | 0.15          | 46-47                         |
| 28.3            | 0.15          | 50                            |
| 30.1            | 2.7           | 55-56                         |
| 33.6            | 0.7           | 57-58                         |
| 35.8            | 0.6           | 63                            |
| 43.4            | 0.05          | 69                            |
| 50.5            | 1.1           | 71-73                         |
| 52.2            | 0.1           | 75-78                         |
| 58.7            | 0.6           | 81-82                         |
| 59.7            | 0.15          | 85-86                         |
| 61.7            | 0.5           | 87-90                         |
| 62.7            | 0.1           | 91-92                         |
| 67.6            | 0.15          | 93-94                         |
| 69.5            | 0.05          | 95-98                         |
| 71.2            | 0.15          | 99-102                        |
| 75.6            | 0.4           | 105-106                       |
| 76.1            | 0.4           | 107-108                       |

TABLE S2: (continued)

| <b>Energy<br/>(meV)</b> | <b><math>\eta</math><br/>(%)</b> | <b>Assigned<br/>calculated mode #</b> |
|-------------------------|----------------------------------|---------------------------------------|
| 77.8                    | 0.3                              | 111-112                               |
| 83.0                    | 0.6                              | 117-121                               |
| 86.4                    | 0.95                             | 123-129                               |
| 93.8                    | 0.1                              | 142-143                               |
| 94.7                    | 0.3                              | 144-146                               |
| 97.3                    | 0.1                              | 151-154                               |
| 100.1                   | 0.1                              | 157-158                               |
| 105.9                   | 0.05                             | 165-168                               |
| 108.7                   | 0.2                              | 169-172                               |
| 136.3                   | 0.7                              | 205-212                               |
| 138.6                   | 0.4                              | 217-218                               |
| 144.1                   | 0.35                             | 225-226                               |
| 146.7                   | 0.55                             | 233-234                               |
| 147.2                   | 0.5                              | 235-236                               |
| 159.4                   | 0.6                              | 239-240                               |
| 160.6                   | 0.15                             | 242-247                               |
| 173.4                   | 0.4                              | 257-258                               |
| 174.4                   | 0.2                              | 260-261                               |
| 176.5                   | 0.15                             | 268                                   |
| 178.7                   | 0.2                              | 271                                   |
| 180.7                   | 0.2                              | 272-274                               |
| 182.4                   | 0.2                              | 276-277                               |
| 185.1                   | 0.15                             | 283-289                               |

- 
- [1] J. P. Perdew, K. Burke, and M. Ernzerhof, [Phys. Rev. Lett. \*\*77\*\*, 3865 \(1996\)](#).
- [2] J.-T. Lü, R. B. Christensen, G. Foti, T. Frederiksen, T. Gunst, and M. Brandbyge, [Phys. Rev. B \*\*89\*\*, 081405 \(2014\)](#).
- [3] T. Gunst, T. Markussen, K. Stokbro, and M. Brandbyge, [Phys. Rev. B \*\*93\*\*, 245415 \(2016\)](#).
- [4] T. Frederiksen, M. Paulsson, M. Brandbyge, and A.-P. Jauho, [Phys. Rev. B \*\*75\*\*, 205413 \(2007\)](#).

- [5] J. Heyd, G. E. Scuseria, and M. Ernzerhof, *J. Chem. Phys.* **118**, 8207 (2003).
- [6] J. Heyd, G. E. Scuseria, and M. Ernzerhof, *J. Chem. Phys.* **124**, 219906 (2006).
- [7] S. L. Dudarev, G. A. Botton, S. Y. Savrasov, C. J. Humphreys, and A. P. Sutton, [Phys. Rev. B \*\*57\*\*, 1505 \(1998\)](#).
- [8] S. Smidstrup, T. Markussen, P. Vancraeyveld, J. Wellendorff, J. Schneider, T. Gunst, B. Verstichel, D. Stradi, P. A. Khomyakov, U. G. Vej-Hansen, M.-E. Lee, S. T. Chill, F. Rasmussen, G. Penazzi, F. Corsetti, A. Ojanperä, K. Jensen, M. L. N. Palsgaard, U. Martinez, A. Blom, M. Brandbyge, and K. Stokbro, [J. Phys. Condens. Matter \*\*32\*\*, 015901 \(2019\)](#).
- [9] M. E. Flatté and J. M. Byers, *Phys. Rev. B* **56**, 11213 (1997).
